# Supplementary material for: The vortex gas scaling regime of baroclinic turbulence
Source: arXiv:2010.10983 source file (2020-10-21)
Supplement: Supplementary file 1 [file SI_Appendix_v4.pdf]

PNAS
www.pnas.org

# Supplementary Information for

## The vortex gas closure of baroclinic turbulence

**Basile Gallet and Raffaele Ferrari**

**Basile Gallet.**
**E-mail: basile.gallet@cea.fr**

### This PDF file includes:

Supplementary text
Fig. S1
References for SI reference citations

## Supporting Information Text

## 1. Equations

We consider the two-layer QG equations (1, 2), as written in the appendix of Thompson & Young (2007), with $\chi = 1$ (drag acting only on the bottom layer) and $\beta = 0$ (constant Coriolis parameter). This value of $\chi$ is not the case considered by Thompson and Young, but is the case considered by Larichev and Held (1995). The potential vorticity (PV) equation in each layer reads:

$$\partial_t q_1 + U\partial_x q_1 + \frac{U}{\lambda^2}\partial_x \psi_1 + J(\psi_1, q_1) = -\nu \boldsymbol{\nabla}^8 q_1 \qquad [1]$$

$$\partial_t q_2 - U\partial_x q_2 - \frac{U}{\lambda^2}\partial_x \psi_2 + J(\psi_2, q_2) = -\nu \boldsymbol{\nabla}^8 q_2 + \text{drag} \qquad [2]$$

where the subscripts 1 and 2 refer respectively to the upper and lower layers, and $\psi_1$ and $\psi_2$ denote the departures of the streamfunctions from the base shear-flow. The expression of the drag term is given below equation [4] of the main document, in terms of the full streamfunction in the bottom layer. One must substitute $\psi_2 \to Uy + \psi_2$ in these expressions to obtain the drag term in terms of the departure of the bottom streamfunction from the base flow, which enters equation [2] above. This substitution does not modify the linear drag term, but some cross terms between $U$ and $\psi_2$ arise in the case of quadratic drag. In practice, however, these terms turn out to be negligible because the eddy velocity is much larger than $U$.

We focus on the case of layers of equal depths, and the PVs are related to the streamfunctions through:

$$q_1 = \boldsymbol{\nabla}^2\psi_1 + \frac{1}{2\lambda^2}(\psi_2 - \psi_1)\,, \qquad [3]$$

$$q_2 = \boldsymbol{\nabla}^2\psi_2 + \frac{1}{2\lambda^2}(\psi_1 - \psi_2)\,. \qquad [4]$$

The barotropic streamfunction is $\psi = (\psi_1 + \psi_2)/2$, while the baroclinic streamfunction is $\tau = (\psi_1 - \psi_2)/2$. The convention here is that the velocity in each layer is $\mathbf{u}_{1;2} = -\boldsymbol{\nabla} \times (\psi_{1;2}\, \mathbf{e}_z)$. The sum and the difference of [1] and [2] lead to the evolution equations for the barotropic and baroclinic streamfunctions:

$$\partial_t(\boldsymbol{\nabla}^2\psi) + J(\psi, \boldsymbol{\nabla}^2\psi) + J(\tau, \boldsymbol{\nabla}^2\tau) + U\partial_x(\boldsymbol{\nabla}^2\tau) = -\nu\boldsymbol{\nabla}^{10}\psi + \text{drag}/2\,, \qquad [5]$$

$$\partial_t[\boldsymbol{\nabla}^2\tau - \lambda^{-2}\tau] + J(\psi, \boldsymbol{\nabla}^2\tau - \lambda^{-2}\tau) + J(\tau, \boldsymbol{\nabla}^2\psi) + U\partial_x[\boldsymbol{\nabla}^2\psi + \lambda^{-2}\psi] = -\nu\boldsymbol{\nabla}^8[\boldsymbol{\nabla}^2\tau - \lambda^{-2}\tau] - \text{drag}/2\,. \qquad [6]$$

We form the energy budget by multiplying [5] by $\psi$ and [6] by $\tau$, before summing the two and averaging over space and time. Neglecting the hyperviscous energy dissipation term and restricting attention to the low-drag regime where $\psi \gg \tau$, we obtain equation [7] of the Letter.

## 2. Numerical runs

In the numerical code, we non-dimensionalize the equations using the spatial scale $L$, where the side-length of the doubly periodic numerical domain is $2\pi L$, and the velocity scale $U$. The dimensionless

equations are:

$$\partial_t q_1 + \partial_x q_1 + \left(\frac{L}{\lambda}\right)^2 \partial_x \psi_1 + J(\psi_1, q_1) = -\tilde{\nu}\boldsymbol{\nabla}^8 q_1 \,, \quad [7]$$

$$\partial_t q_2 - \partial_x q_2 - \left(\frac{L}{\lambda}\right)^2 \partial_x \psi_2 + J(\psi_2, q_2) = -\tilde{\nu}\boldsymbol{\nabla}^8 q_2 + \tilde{\text{drag}} \,, \quad [8]$$

where $\tilde{\nu} = \nu/(UL^7)$, the dimensionless time is in units of $L/U$, the dimensionless PVs are in units of $U/L$, and the dimensionless streamfunctions are in units of $UL$.

Equations [7-8] are time-stepped using a standard pseudo-spectral method, with a fourth-order Runge-Kutta time-stepping scheme and an adaptive time-step. The linear terms are treated implicitly, except for the drag term that is treated explicitly for both linear and quadratic drag. We apply de-aliasing using the 1/2 rule, because of the cubic nonlinearity arising in the quadratic-drag term. The following tables contain the parameter values of the data points presented in the Letter:

| $\kappa_* = \kappa\lambda/U$ | 1.0 | 0.6 | 0.3 | 0.2 | 0.1 |
|---|---|---|---|---|---|
| Resolution | $1024^2$ | $1024^2$ | $1024^2$ | $1024^2$ | $4096^2$ |
| $\lambda/L$ | 0.01 | 0.01 | 0.01 | 0.01 | 0.0025 |
| $\tilde{\nu} = \nu/(UL^7)$ | $7.8\,10^{-16}$ | $7.8\,10^{-16}$ | $7.8\,10^{-16}$ | $7.8\,10^{-16}$ | $4.8\,10^{-20}$ |

| $\mu_* = \mu\lambda$ | 1.0 | 0.3 | 0.1 | 0.03 | 0.01 | 0.003 | 0.001 |
|---|---|---|---|---|---|---|---|
| Resolution | $512^2$ | $512^2$ | $512^2$ | $512^2$ | $512^2$ | $512^2$ | $1024^2$ |
| $\lambda/L$ | 0.02 | 0.02 | 0.02 | 0.02 | 0.02 | 0.02 | 0.02 |
| $\tilde{\nu} = \nu/(UL^7)$ | $10^{-13}$ | $10^{-13}$ | $10^{-13}$ | $10^{-13}$ | $10^{-13}$ | $10^{-13}$ | $10^{-14}$ |

## 3. Heat transport by a vortex dipole

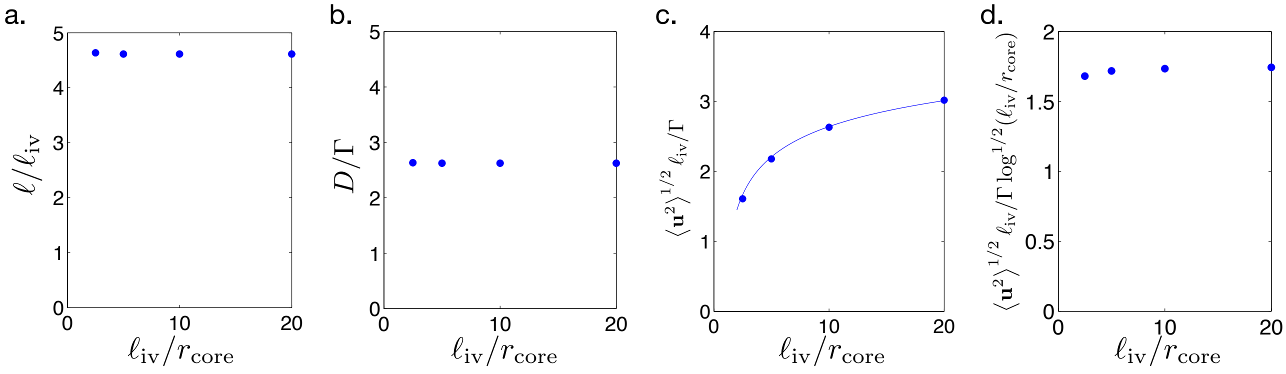


**Fig. S1. Heat transport by a single dipole.** Diagnosed dimensionless mixing length (a), diffusivity (b), and rms velocity (c) for a single dipole of vortices of various core radii, at the end time of the numerical integration. The solid line is $1.74\ \log^{1/2}(\ell_{iv}/r_{core})$. Panels (c) and (d) make it clear that $\langle \mathbf{u}^2 \rangle^{1/2}/V$ scales as $\log^{1/2}(\ell_{iv}/r_{core})$.

We consider the advection-diffusion equation [10] of the main document, when the barotropic vorticity $\zeta$ consists in a self-advecting dipole of Gaussian vortices (5):

$$\zeta(x,y,t) = \Gamma e^{-\frac{(x-X_1)^2+(y-Y_1)^2}{r_{core}^2}} - \Gamma e^{-\frac{(x-X_2)^2+(y-Y_2)^2}{r_{core}^2}} \,, \qquad \nabla^2\psi = \zeta(x,y,t) \,, \quad [9]$$

where the coordinates of the vortex centers depend on time:

$$X_1 = -\ell_{iv}/2\,; \qquad Y_1 = \pi\ell_{iv} + \frac{\Gamma}{2\pi\ell_{iv}}t\,; \qquad X_2 = \ell_{iv}/2\,; \qquad Y_2 = \pi\ell_{iv} + \frac{\Gamma}{2\pi\ell_{iv}}t\,. \quad [10]$$

We integrate the advection-diffusion equation numerically over the time interval $t \in [0, 2\pi {\ell_{\rm iv}}^2/\Gamma]$, starting from the initial condition $\tau = 0$. The domain size is $(2\pi\ell_{\rm iv})^2$ with periodic boundary conditions, which seems sufficient to avoid boundary effects. We perform this numerical integration for several values of the core radius $r_{\rm core}$, at very low hyperviscosity. At the end of each numerical integration, we estimate the typical mixing length and diffusivity by integrating $\tau^2$ and $\psi_x\tau/U$ over the domain, and dividing by $\ell_{iv}^2$. This yields estimates of the averages in the vicinity of the dipole. More precisely, we evaluate the scaling behaviors of $\ell$, $D$ and of the rms velocity through:

$$\ell^2 \sim \frac{1}{U^2\ell_{iv}^2}\iint \tau^2 \,\mathrm{d}x\mathrm{d}y\,, \qquad [11]$$

$$D \sim \frac{1}{U\ell_{iv}^2}\iint \psi_x\tau \,\mathrm{d}x\mathrm{d}y\,, \qquad [12]$$

$$\left\langle \mathbf{u}^2 \right\rangle \sim \frac{1}{\ell_{iv}^2}\iint |\boldsymbol{\nabla}\psi|^2 \,\mathrm{d}x\mathrm{d}y\,, \qquad [13]$$

where the integrals are over the entire square domain, $(x, y) \in [0, 2\pi\ell_{\rm iv}]^2$. We show these diagnosed quantities in figure S1 for vortices of different core sizes. It is apparent that $\ell/\ell_{\rm iv}$ and $D/\Gamma$ are constant and independent of $r_{\rm core}$, whereas $\langle \mathbf{u}^2\rangle^{1/2}/V$ behaves as $\log^{1/2}(\ell_{\rm iv}/r_{\rm core})$.

## References


1. R. Salmon, Lectures on geophysical fluid dynamics, *Oxford University Press*, 1st edition (1998).
2. G.K. Vallis, Atmospheric and oceanic fluid dynamics: fundamentals and large-scale circulation, *Cambridge University Press*, 2nd edition (2017).
3. A.F. Thompson, W.R. Young, Two-layer baroclinic eddy heat fluxes: zonal flows and energy balance, *J. Atmospheric Sci.*, **64**, 3214-3231 (2007).
4. V. Larichev, I.M. Held, Eddy amplitudes and fluxes in a homogeneous model of fully developed baroclinic instability, *J. Phys. Oceanogr.* **25**, 2285-2297 (1995).
5. P.G. Saffman, Vortex dynamics, *Cambridge University Press* (1992).
